# Supplementary material for: Metal Price Spike Prediction via a Neurosymbolic Ensemble Approach
Source: arXiv:2410.12785 source file (2024-10-16)
Supplement: Supplementary file 1 [file 1_model_evaluation.tex]

\newcommand{\emptyroweval}{\multicolumn{4}{c}{} \\}

\begin{table}
\centering
\begin{tabular}{|c|c|c|c|}
\hline
Model & Precision & Recall & F1\\
\hline
CNN  (12) & 0.82 & \underline{0.65} & \underline{0.73}\\
ATTN (8) & \underline{\textbf{0.94}} & 0.19 & 0.32\\

\hline
CNN  (12) (EDCR) & 0.80 (-2.15\%) & \textbf{0.85} (+29.41\%) & 0.83 (+13.24\%)\\
ATTN (8) (EDCR) & \textbf{0.94} (0.0\%) & 0.19 (0.0\%) & 0.32 (0.0\%)\\

\hline
\emptyroweval
\end{tabular}

\caption{Model Evaluation Results for Cobalt. Using the MPSCRuleLearn algorithm. Filtering by Top F1}
\end{table}
\begin{table}
\centering
\begin{tabular}{|c|c|c|c|}
\hline
Model & Precision & Recall & F1\\
\hline
CNN  (12) & 0.82 & \underline{0.65} & \underline{0.73}\\
ATTN (8) & \underline{\textbf{0.94}} & 0.19 & 0.32\\

\hline
CNN  (12) (EDCR) & 0.85 (+3.0\%) & \textbf{0.78} (+19.61\%) & \textbf{0.81} (+11.63\%)\\
ATTN (8) (EDCR) & \textbf{0.94} (0.0\%) & 0.19 (0.0\%) & 0.32 (0.0\%)\\

\hline
\emptyroweval
\end{tabular}
\caption{Model Evaluation Results for Cobalt. Using the MPSCRuleLearn algorithm. Filtering by Threshold}
\end{table}
\begin{table}
\centering
\begin{tabular}{|c|c|c|c|}
\hline
Model & Precision & Recall & F1\\
\hline
ATTN (2) & 0.78 & 0.74 & \underline{0.76}\\
CNN  (3) & 0.52 & \underline{0.78} & 0.62\\
CNN  (4) & \underline{\textbf{0.83}} & 0.52 & 0.64\\

\hline
ATTN (2) (EDCR) & 0.79 (+0.5\%) & 0.76 (+2.33\%) & \textbf{0.77} (+1.43\%)\\
CNN  (3) (EDCR) & 0.53 (+0.69\%) & \textbf{0.84} (+8.89\%) & 0.65 (+3.84\%)\\
CNN  (4) (EDCR) & \textbf{0.83} (0.0\%) & 0.52 (0.0\%) & 0.64 (0.0\%)\\

\hline
\emptyroweval
\end{tabular}

\caption{Model Evaluation Results for Copper. Using the MPSCRuleLearn algorithm. Filtering by Top F1}
\end{table}
\begin{table}
\centering
\begin{tabular}{|c|c|c|c|}
\hline
Model & Precision & Recall & F1\\
\hline
ATTN (2) & 0.78 & 0.74 & \underline{0.76}\\
CNN  (3) & 0.52 & \underline{0.78} & 0.62\\
CNN  (4) & \underline{0.83} & 0.52 & 0.64\\

\hline
ATTN (2) (EDCR) & 0.79 (+0.5\%) & 0.76 (+2.33\%) & \textbf{0.77} (+1.43\%)\\
CNN  (3) (EDCR) & 0.53 (+0.69\%) & \textbf{0.84} (+8.89\%) & 0.65 (+3.84\%)\\
CNN  (4) (EDCR) & \textbf{0.85} (+1.54\%) & 0.57 (+10.0\%) & 0.68 (+6.6\%)\\

\hline
\emptyroweval
\end{tabular}
\caption{Model Evaluation Results for Copper. Using the MPSCRuleLearn algorithm. Filtering by Threshold}
\end{table}
\begin{table}
\centering
\begin{tabular}{|c|c|c|c|}
\hline
Model & Precision & Recall & F1\\
\hline
CNN  (1) & 0.52 & 0.65 & \underline{0.58}\\
RNN  (4) & 0.20 & \underline{0.99} & 0.33\\
CNN  (2) & \underline{\textbf{0.86}} & 0.17 & 0.28\\

\hline
CNN  (1) (EDCR) & 0.53 (+3.19\%) & 0.79 (+21.74\%) & \textbf{0.64} (+10.67\%)\\
RNN  (4) (EDCR) & 0.20 (+0.87\%) & \textbf{1.00} (+1.43\%) & 0.33 (+0.96\%)\\
CNN  (2) (EDCR) & \textbf{0.86} (0.0\%) & 0.17 (+0.0\%) & 0.28 (0.0\%)\\

\hline
\emptyroweval
\end{tabular}
\caption{Model Evaluation Results for Magnesium. Using the MPSCRuleLearn algorithm. Filtering by Top F1}
\end{table}
\begin{table}
\centering
\begin{tabular}{|c|c|c|c|}
\hline
Model & Precision & Recall & F1\\
\hline
CNN  (1) & 0.52 & 0.65 & \underline{0.58}\\
RNN  (4) & 0.20 & \underline{0.99} & 0.33\\
CNN  (2) & \underline{\textbf{0.86}} & 0.17 & 0.28\\

\hline
CNN  (1) (EDCR) & 0.53 (+3.19\%) & 0.79 (+21.74\%) & \textbf{0.64} (+10.67\%)\\
RNN  (4) (EDCR) & 0.19 (-0.52\%) & \textbf{1.00} (+1.43\%) & 0.33 (-0.2\%)\\
CNN  (2) (EDCR) & \textbf{0.86} (0.0\%) & 0.17 (+0.0\%) & 0.28 (0.0\%)\\

\hline
\emptyroweval
\end{tabular}
\caption{Model Evaluation Results for Magnesium. Using the MPSCRuleLearn algorithm. Filtering by Threshold}
\end{table}
\begin{table}
\centering
\begin{tabular}{|c|c|c|c|}
\hline
Model & Precision & Recall & F1\\
\hline
ATTN (5) & 0.59 & 0.48 & \underline{0.53}\\
CNN  (6) & 0.37 & \underline{0.57} & 0.45\\
ATTN (8) & \underline{0.66} & 0.38 & 0.48\\

\hline
ATTN (5) (EDCR) & 0.60 (+1.38\%) & 0.59 (+24.14\%) & \textbf{0.60} (+12.85\%)\\
CNN  (6) (EDCR) & 0.40 (+6.42\%) & \textbf{0.69} (+20.0\%) & 0.50 (+11.38\%)\\
ATTN (8) (EDCR) & \textbf{0.68} (+2.82\%) & 0.41 (+8.7\%) & 0.51 (+6.48\%)\\

\hline
\emptyroweval
\end{tabular}
\caption{Model Evaluation Results for Nickel. Using the MPSCRuleLearn algorithm. Filtering by Top F1}
\end{table}
\begin{table}
\centering
\begin{tabular}{|c|c|c|c|}
\hline
Model & Precision & Recall & F1\\
\hline
ATTN (5) & 0.59 & 0.48 & \underline{0.53}\\
CNN  (6) & 0.37 & \underline{0.57} & 0.45\\
ATTN (8) & \underline{\textbf{0.66}} & 0.38 & 0.48\\

\hline
ATTN (5) (EDCR) & 0.61 (+2.59\%) & 0.56 (+17.24\%) & \textbf{0.58} (+10.23\%)\\
CNN  (6) (EDCR) & 0.37 (-0.12\%) & \textbf{0.74} (+28.57\%) & 0.49 (+9.5\%)\\
ATTN (8) (EDCR) & \textbf{0.66} (+0.21\%) & 0.44 (+17.39\%) & 0.53 (+10.49\%)\\

\hline
\emptyroweval
\end{tabular}
\caption{Model Evaluation Results for Nickel. Using the MPSCRuleLearn algorithm. Filtering by Threshold}
\end{table}
